# Supplementary material for: TAHB: A Comprehensive Benchmark for Text-Attributed Hypergraph Learning
Source: arXiv:2608.15055 source file (2026-08-15)
Supplement: Supplementary file 1 [file s8_appendix.tex]

\section{Datasets}
\subsection{Dataset Description}
\noindent \textbf{Dataset Format.}
\noindent \textbf{E-commerce.}
\noindent \textbf{Academic.}
\noindent \textbf{Political.}
\noindent \textbf{Movie.}

\subsection{Dataset Analysis}
\input{TAHB_Apps/Tabs/Table6}




\subsection{Dataset License}
The datasets are released under the MIT License. For detailed licensing and usage information, please refer to the corresponding GitHub repository

% 여기까지 진행함 여까지가 A임




\subsection{Datasets}\label{A}
In this section, we describe the detailed settings of our experiments.

\noindent \textbf{Reproducibility.}
The experiments are conducted on the Linux server equipped with an AMD 7960X, 2TB NVMe SSD, 128GB DDR5 memory, and GeForce RTX A6000(48G).
For HRL methods, we use the source codes provided by the authors of the original papers~\cite{wan23:iclr, wan23:icml,hua21:ijcai,ci21:iclr,fen19:aaai,yad19:neurips,lee23:aaai,wei22:nips,du22:bd,kim24:iclr,zhe22:nips,hou23:www,li23:kdd}.
For parameters for each method, we use the best setting found via extensive grid search in the ranges suggested in its respective paper.
% \footnote{We have released the code of {\hgc} and datasets at the link https://anonymous.4open.science/r/HyperGC/main.py} 
We carefully tune the hyperparameters of our {\hgc} via grid search over the following ranges.
The loss weights $\omega_{(n)}$, $\omega_{(h)}$, $\omega_{ce}$ and $\omega_{cl}$ are selected from [$2^{-4}, 2^{-3}, \dots, 2^{4}$].
The temperature parameters for contrastive loss, $\tau_{n}$ and $\tau_{h}$, are chosen from [$0.1, 0.2, \dots, 1.0$].
For hypergraph augmentation, the feature, incidence, and hyperedge masking rates are all varied within [$0.1, 0.2, \dots, 1.0$].
The hidden dimension is selected from [$2^6, 2^7, \dots, 2^{10}$], and the learning rate is from [$10^{-5}, 5 \times 10^{-5}, 10^{-4}, 5 \times 10^{-4}, 10^{-3}$].
The weight decay is tuned over [$10^{-5}, 5 \times 10^{-5}, 10^{-4}, 5 \times 10^{-4}$].
The numbers of encoder layers and LSTM layers are selected from [$2^0, 2^1, \dots, 2^4$].
\input{TAHB_Apps/Tabs/Table7}
\input{TAHB_Apps/Tabs/Table8}
\vspace{1mm}
\noindent \textbf{Datasets.}
In this paper, we use 11 real-world hypergraph datasets collected from diverse domains, including co-citation (Cora~\cite{yad19:neurips}, Citeseer~\cite{yad19:neurips}, and PubMed~\cite{yad19:neurips}), co-authorship (Cora-CA~\cite{yad19:neurips}, DBLP-P~\cite{yad19:neurips}, DBLP-A~\cite{wan19:www}, and AMiner~\cite{zha19:kdd}), computer graphics (MN-40~\cite{wu15:cvpr}), movie–actor relationships (IMDB~\cite{wan19:www}), news content (20News~\cite{kel17}), and political membership affiliations (House~\cite{ci21:iclr}).
\begin{itemize}[leftmargin=*]
    \item \textbf{Cora, Citeseer, and Pubmed}: These three datasets are co-citation datasets where each node denotes a publication, and each hyperedge consists of a group of papers that are jointly cited by a single citing paper. Node features are bag-of-words representations of the publication text, and node classes indicate their academic categories.
    \item \textbf{Cora-CA, DBLP-P, DBLP-A, and AMiner}: These four datasets are co-authorship datasets where each node represents a publication, and each hyperedge consists of a group of papers that are written by the same author. Node features and node classes are defined in the same way as in the co-citation datasets.
    \item \textbf{MN-40}: This dataset is a computer graphic dataset where each node represents a visual object, and each hyperedge each hyperedge is a synthetic hyperedge constructed from a $k$-nearest neighbor (k-NN) graph built using the feature representations of the data points. Node features are vectors of the corresponding visual objects. Node classes indicate the object categories. 
    \item \textbf{IMDB}: This dataset is a movie–actor relational dataset where each node represents a movie, and each hyperedge consists of the set of movies (filmography) associated with a single actor. Node features are bag-of-words of the plot of the corresponding movie. Node class indicates the genre of the movie.
    \item \textbf{20News}: This dataset is a news dataset where each node represents a document of 20 newsgroups and each hyperedge consists of the set of documents containing a particular word. Node features are TF-IDF representations of news messages of the corresponding news document. Node class indicates the category of the corresponding news document.
    \item \textbf{House}: This dataset is a political membership dataset where each node represents a member of the US House of Representatives and each hyperedge consists of members belonging to the same committee. Node features are generated by adding noise to the one-hot encoded label vector. Node class indicates the political party of the corresponding member.   
\end{itemize}

\begin{figure*}[t]
\centering
\includegraphics[width=0.95\textwidth]{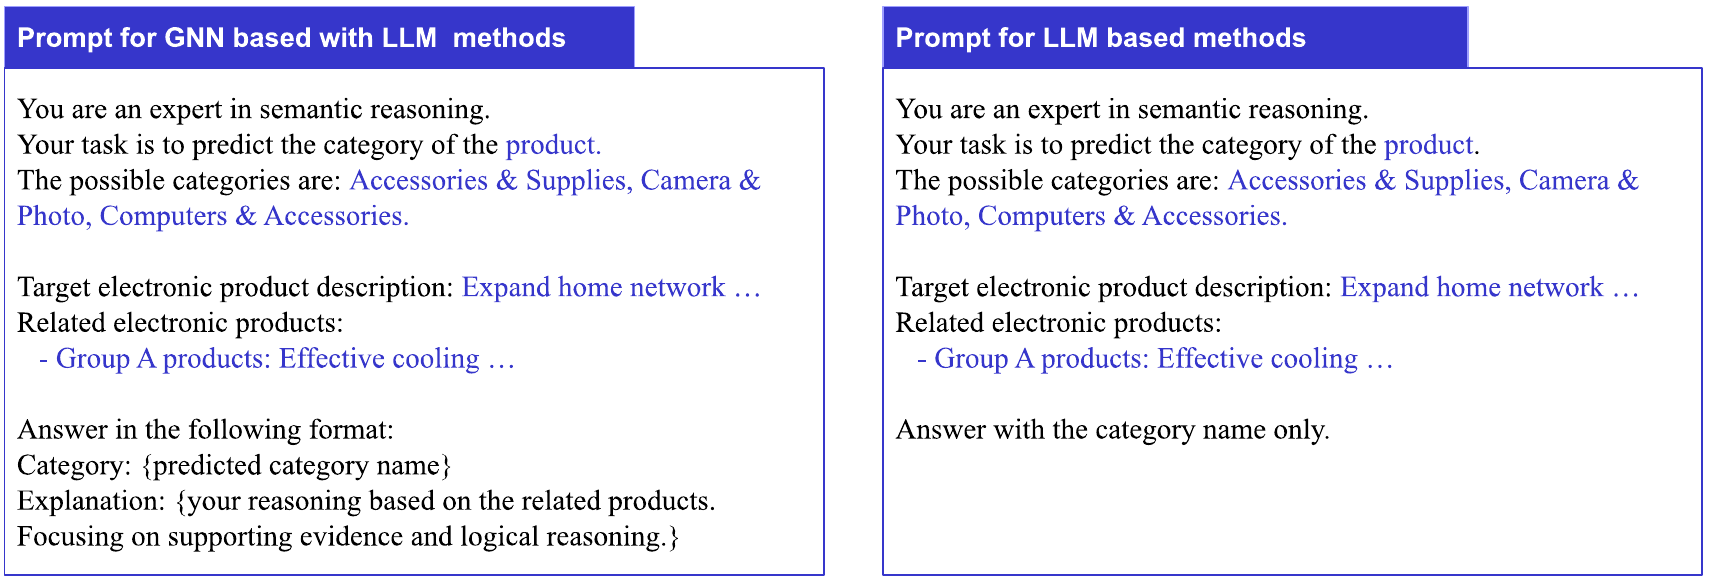}
\vspace{-3mm}
\caption{Example prompts used in LLM-utilized paradigms. The examples are constructed for the Amazon Electronics dataset, and inputs whose values vary across different datasets are highlighted in blue.} \label{fig_6}
\vspace{-3mm}
\label{fig7}
\end{figure*}
%\input{TAHB_Apps/Tabs/Table9}
%\input{TAHB_Apps/Tabs/Table10}
